# Supplementary material for: PointNet4D: A Lightweight 4D Point Cloud Video Backbone for Online and Offline Perception in Robotic Applications
Source: arXiv:2512.01383 source file (2025-12-01)
Supplement: Supplementary file 1 [file _supplementary.tex]

\def\paperTitle{Paper Title}

\def\authorBlock{
    Yunze Liu \\
    % Author 3 \\
    Institute \\
    {\tt\small \{email, addresses\}@inst.edu}
}

% Compilation vars
\newif\ifreview \newcommand{\review}{\reviewtrue}
\newif\ifarxiv 
\newif\ifcamera 
\newif\ifrebuttal 

\review % \review OR \cameraready

\documentclass[10pt,twocolumn,letterpaper]{article}
\ifreview \usepackage[review]{cvpr} \fi
\ifarxiv \usepackage[pagenumbers]{cvpr} \fi
\ifrebuttal \usepackage[rebuttal]{cvpr} \fi
\ifcamera \usepackage{cvpr} \fi

%% PACKAGES (also see cvpr_header.tex)

\usepackage{graphicx}	
\usepackage{amsmath}	
\usepackage{amssymb}	
\usepackage{booktabs}
\usepackage{times}
\usepackage{microtype}
\usepackage{epsfig}
\usepackage{caption}
\usepackage{float}
\usepackage{placeins}
\usepackage{color, colortbl}
\usepackage{xcolor}
\usepackage{stfloats}
\usepackage{enumitem}
\usepackage{tabularx}
\usepackage{xstring}
\usepackage{multirow}
\usepackage{xspace}
\usepackage{url}
\usepackage{subcaption}

\usepackage[hang,flushmargin]{footmisc}
% Include other packages here, before hyperref.
\usepackage{graphicx}
\usepackage{amsmath}
\usepackage{amssymb}
\usepackage{booktabs}
\usepackage{algorithmic} %
\usepackage{color,xcolor}
\usepackage{amsmath}
\usepackage{xspace}
\usepackage{multirow}
\definecolor{shapecolor}{rgb}{0.0,0.5,0.0}
\definecolor{mygray}{gray}{.9}

\usepackage{hyperref}       %
\usepackage{url}            %
\usepackage{booktabs}       %
\usepackage{graphicx}
\usepackage{amsfonts}       %
\usepackage{nicefrac}       %
\usepackage{microtype}      %
\usepackage{xcolor}         %
\usepackage{algorithm}
\usepackage{tabularx}

\newcommand{\app}{\raise.17ex\hbox{$\scriptstyle\sim$}}

% It is strongly recommended to use hyperref, especially for the review version.
% hyperref with option pagebackref eases the reviewers' job.
% Please disable hyperref *only* if you encounter grave issues, e.g. with the
% file validation for the camera-ready version.
%
% If you comment hyperref and then uncomment it, you should delete
% ReviewTempalte.aux before re-running LaTeX.
% (Or just hit 'q' on the first LaTeX run, let it finish, and you
%  should be clear).
\usepackage[pagebackref,breaklinks,colorlinks]{hyperref}
\usepackage[table,xcdraw]{xcolor}

% Support for easy cross-referencing
\usepackage[capitalize]{cleveref}
\crefname{section}{Sec.}{Secs.}
\Crefname{section}{Section}{Sections}
\Crefname{table}{Table}{Tables}
\crefname{table}{Tab.}{Tabs.}
% Unfortunately, this package interferes with arxiv's stamp
\ifcamera \usepackage[accsupp]{axessibility} \fi

%% MACROS

% \newcommand{\authorname}[1]{{\textcolor{blue}{[Author: #1]}}}
% ...

% \newcommand{\commandname}{string\xspace}
% \definecolor{colorname}{rgb}{0.92,0.49,0.19}

% General

\ifarxiv  \fi

% Reviewer commands (1 to 5), e.g. \R{1}, \R{2}
\newcommand{\R}[1]{{%
    \textbf{%
        \ifstrequal{#1}{1}{\textcolor{red}{R#1}}{%
        \ifstrequal{#1}{2}{\textcolor{blue}{R#1}}{%
        \ifstrequal{#1}{3}{\textcolor{magenta}{R#1}}{%
        \ifstrequal{#1}{4}{\textcolor{teal}{R#1}}{%
                           \textcolor{cyan}{R#1}%
        }}}}%
    }%
}}
  % Add packages to _macros.tex

%% For cross-referencing labels between documents
\usepackage{xr-hyper}

\makeatletter
\newcommand*{\addFileDependency}[1]{
  \typeout{(#1)}
  \@addtofilelist{#1}
  \IfFileExists{#1}{}{\typeout{No file #1.}}
}

\makeatother
\newcommand*{\myexternaldocument}[1]{
    \externaldocument{#1}
    \addFileDependency{#1.tex}
    \addFileDependency{#1.aux}
}

\definecolor{cvprblue}{rgb}{0.21,0.49,0.74}
\usepackage[pagebackref,breaklinks,colorlinks,allcolors=cvprblue]{hyperref}
\usepackage[capitalize]{cleveref}
\crefname{section}{Sec.}{Secs.}
\crefname{table}{Table}{Tables}
\crefname{figure}{Fig.}{Figs.}

\ifarxiv \crefname{appendix}{App.}{Apps.}
\else \crefname{appendix}{Suppl.}{Suppls.} \fi

\frenchspacing

\myexternaldocument{_main}
\begin{document}

%% TITLE
\title{\paperTitle}
\author{\authorBlock}
\maketitlesupplementary

\appendix
\input{12_appendix}

{\small
\bibliographystyle{ieeenat_fullname}
\bibliography{11_references}
}

\end{document}
